# Supplementary material for: Economic impact of biomarker-based aging interventions on healthcare costs and individual value
Source: arXiv:2503.20357 source file (2025-03-26)
Supplement: Supplementary file 1 [file appendix.tex]

\section{Background: Key Clinical Trials in Longevity Medicine}

To inform our approach, we examined major clinical trials in longevity medicine, evaluating their endpoints and potential relevance to evidence generation in geroscience. These trials employed diverse interventions and endpoints, providing valuable insights for our model development.

\subsection{Nutritional and Exercise Interventions}

\textbf{DO-HEALTH Trial} evaluated the combined effects of vitamin D3, omega-3 fatty acids, and strength home exercise. Results demonstrated that the combined intervention significantly decreased odds of becoming pre-frail compared to control groups. Additionally, daily high-dose vitamin D3 plus omega-3s, combined with home exercise, showed cumulative reduction in cancer risk among generally healthy and active adults aged 70 years and above who were largely vitamin D-replete.

\textbf{CALERIE} (Comprehensive Assessment of Long-term Effects of Reducing Intake of Energy) investigated caloric restriction (CR) versus control conditions. Primary outcomes included changes in core body temperature, resting metabolic rate corrected for body composition changes, and measurements from baseline to 12 and 24 months. Results generally favored the intervention, supporting caloric restriction as a potential longevity strategy.

\textbf{GENERATION-100} compared exercise interventions (moderate-intensity continuous training and high-intensity interval training) with control groups, using mortality as the primary endpoint. While combined MICT and HIIT showed no significant effect on all-cause mortality compared with recommended physical activity levels, researchers observed a lower all-cause mortality trend after HIIT compared with controls and MICT.

\subsection{Pharmaceutical Interventions}

\textbf{ASPREE Trial} compared 100 mg enteric-coated aspirin with placebo, using a composite primary endpoint of death from any cause, incident dementia, or persistent physical disability. Results indicated that aspirin did not prevent disability-free survival but increased major bleeding risk compared with placebo.

\textbf{Metformin for Preventing Frailty in High-risk Older Adults} evaluated metformin versus placebo with frailty as the primary outcome measure. Results are not yet available but may provide valuable insights into pharmaceutical approaches to frailty prevention.

\textbf{mTOR\_ANZ} compared placebo with BEZ235 and BEZ235 plus everolimus (RAD001). The primary outcome was the percentage of subjects with one or more laboratory-confirmed respiratory tract infections through Week 16, investigating the immunomodulatory effects of mTOR inhibition.

\textbf{DASATINIB/QUERCETIN} trial compared the senolytic combination of Dasatinib plus Quercetin with control groups, utilizing epigenetic age testing as the primary outcome. Results are pending but represent an important investigation into senolytics as a longevity intervention.

\textbf{Topical-RAPA} evaluated rapamycin topical ointment versus placebo, measuring changes in epigenetic markers and differences in epigenetic clock ages as primary outcomes.

\textbf{SGLT2 Inhibition in Older Obese Adults With Pre-diabetes (SGLT2i)} is comparing Dapagliflozin 10 mg with nutritional counseling, using AGE-RAGE measurement in urine as the primary outcome. This study is ongoing.

\subsection{Biological Interventions}

\textbf{MoTrPAC} compared endurance training with resistance training, examining transcriptome, metabolome, lipidome, proteome, epigenome, and genomic influences in muscle. Results are available in animal models.

\textbf{TRIIM-X} is comparing TRIIM Treatment with an active control, with primary outcomes including epigenetic age, thymus regeneration, safety, and tolerability. This study is ongoing with expected completion in 2024.

\textbf{PLASMA} compared plasma treatment with control groups, measuring safety, tolerability, and protocol compliance. Results indicated acceptable safety and tolerability profiles.

These trials collectively illustrate the diverse approaches to longevity intervention and the varied endpoints employed to measure efficacy. Our work builds upon these foundations, utilizing frailty-related endpoints and epigenetic markers to model potential economic and clinical impacts of longevity-focused interventions.
